# Supplementary material for: Stein Variational Message Passing for Continuous Graphical Models
Source: arXiv:1711.07168 source file (2018-06-07)
Supplement: Supplementary file 1 [file appendix_text.tex]

\appendix
\numberwithin{equation}{section}

\section{ Proof of Theorem \ref{thm:optimal} .}

\begin{proof}
Using the reproducing property of $\H_i$, 
$$
\begin{aligned}
&\E_{x\sim q}[\stein_p f(x)] = \langle f, \E_{x \sim q}[\stein_p \odot \K(x, \cdot)] \rangle_{\H} \\
% &= \sum_{i=1}^d \langle f, \E_{x \sim q}[ \partial_{x_i}\log p(x)\k_i(x,\cdot) + \partial_{x_i}\k_i(x,\cdot)] \rangle_{\H_i} \\
% &= \sum_{i=1}^d \langle f_i, \E_{x \sim q}[ \stein_{p}^{x_i}k_i(x,\cdot)] \rangle_{\H_i} \\
\end{aligned}
$$
Let us denote the function $\phi^*(\cdot) =\E_{x \sim q}[\stein_p \odot \vv k(x,\cdot)]$.
Then the optimization of the Stein Discrepancy is framed into
$$
\max_f \langle f, \phi^* \rangle_{\H}, ~~s.t.~~ ||f||_{\H} \le 1.
$$

It is straightforward to see that the optimal $f$ should be a normalized version of $\phi^*$,
that is $f = \phi^* \slash ||\phi^*||_{\H}$.
Similarly to previous work \citep{liu2016kernelized,chwialkowski2016kernel},
we obtain a closed form solution of Stein discrepancy $\S(q~||~p)$
by substituting $\phi^* \slash ||\phi^*||_{\H}$
for the $\phi$
in the definition of Stein discrepancy \eqref{equ:ksd_prob}.
\end{proof}

\section{Proof of Proposition \ref{thm:wdistance}.}
\begin{proof}

First, we denote the update in our algorithm by $T_{q,p}(x) = x + \epsilon \E_{y \sim q}[\stein_p^y \odot \vv k(x,y)]$. Then we have the following equation.

\begin{equation}\label{eq:update_diff}
\begin{aligned}
&|\frac{T_{\hat{q}_s^n,p}(u) - T_{q_s^\infty,p}(v)}{u - v}| \\
&= |1 + \epsilon \frac{\E_{x \sim \hat{q}_s^n}g(x,u) - \E_{z \sim q_s^\infty}g(z,v)}{u-v}| \\
&= 1 + \frac{\epsilon}{|u - v|} 
| [\E_{x \sim \hat{q}_s^n}g(x,u) - \E_{x \sim \hat{q}_s^n}g(x,v)] \\
&  - [\E_{x \sim \hat{q}_s^n}g(x,v) - \E_{z \sim q_s^\infty}g(z,v)]  | \\
\end{aligned}
\end{equation}

Since $g(x,y):=\stein_p^x \odot \K(x,y)$ is Lipschitz continuous jointly on $(x,y)$, the following ineuqality holds for some constant $\mathcal{L}$.

\begin{equation}\label{eq:lips}
\begin{aligned}
|\E_{x \sim \hat{q}_s^n}g(x,u) - \E_{x\sim \hat{q}_s^n}g(x,v)|
&\leqslant \mathcal{L} |u - v|
\end{aligned}
\end{equation}

By replacing in \eqref{eq:update_diff} with \eqref{eq:lips}, we obtain the following inquality
$$
|\frac{T_{\hat{q}_s^n,p}(u) - T_{q_s^\infty,p}(v)}{u - v}| \leqslant 1 + \epsilon\mathcal{L} + \epsilon|\frac{h_s(v)}{u-v}|
$$

where $h_s(v) = \E_{x \sim \hat{q}_s^n}g(x,v) - \E_{x\sim q_s^\infty}g(x,v)$. 
It could be easily verified that $h_s(v)$ is also Lipschitz continuous with constant $2\mathcal{L}$. 
Now for any probability measure $\gamma \in \Gamma(\hat{q}_s^n,q_s^\infty)$,
we have the following results

$$
\begin{aligned}
&\int (1 + \epsilon\mathcal{L} + \epsilon|\frac{h_s(v)}{u-v}|)|u-v|d\gamma(u,v)\\
\geqslant & \int |\frac{T_{\hat{q}_s^n,p}(u) - T_{q_s^\infty,p}(v)}{u - v}| \cdot |u-v| d\gamma(u,v)\\
= & \int |T_{\hat{q}_s^n,p}(u) - T_{q_s^\infty,p}(v)|d\gamma(u,v) \\
= & \int |x - y|d \gamma(T_{\hat{q}_s^n,p}^{-1}(x),T_{q_s^\infty,p}^{-1}(y))\\
= & \int |x - y|d \gamma'(x,y)
\end{aligned}
$$

Note that here $\gamma'(x,y) = \gamma(T_{\hat{q}_s^n,p}^{-1}(x),T_{q_s^\infty,p}^{-1}(y))$. 
For properly small $\epsilon$,
both $T_{\hat{q}_s^n,p}$ and $T_{q_s^\infty,p}$ are invertible.

Furthermore, 
we denote the transformation of probability distributions by $\Phi : q \mapsto \Phi(q)$ where $\Phi(q)$ is defined to be the distribution of variable $T_{q,p}(x)$ with $x \sim q$.
Then we have $\gamma' \in \Gamma(\Phi(\hat{q}_s^n), \Phi(q_s^\infty))$ by the transformation of random variables. On the other hand, it holds that
$$
\begin{aligned}
&\int (1 + \epsilon\mathcal{L} + \epsilon|\frac{h_s(v)}{u-v}|)|u-v|d\gamma(u,v)\\
= & (1 + \epsilon\mathcal{L})\int|u-v|d\gamma(u,v) + \epsilon \int|h_s(v)|d\gamma(u,v)\\
\end{aligned}
$$
For the second term, it can be rewritten as an expectation.
$$
\begin{aligned}
&\int|h_s(v)|d\gamma(u,v)\\
=& \int|h_s(v)|dq_s^\infty(v) = \E_{v\sim q_s^\infty}|h_s(v)|
\end{aligned}
$$

Then we have that for arbitrary $\gamma \in \Gamma(\hat{q}_s^n,q_s^\infty)$, there exists a probability measure $\gamma' \in \Gamma(\Phi(\hat{q}_s^n), \Phi(q_s^\infty))$ such that
$$
\begin{aligned}
&(1 + \epsilon\mathcal{L})\int|u-v|d\gamma(u,v) + \epsilon \E_{v\sim q_s^\infty}|h(v)| \\
&\quad\quad \geqslant \int |x-y|d\gamma'(x,y)\\
\end{aligned}
$$

Considering the definiton of $L1-$Wasserstein distance, 
the above inequality actually reveals the relationship between two $L1-$Wasserstein distances $\mathcal{W}_1(\hat{q}_s^n,q_s^\infty)$ and $\mathcal{W}_1(\Phi(\hat{q}_s^n),\Phi(q_s^\infty))$ as follows. 
$$
\begin{aligned}
& (1+\epsilon\mathcal{L})\mathcal{W}_1(\hat{q}_s^n,q_s^\infty) + \E_{v\sim q_s^\infty}|h_s(v)|\\
& \quad\quad \geqslant \mathcal{W}_1(\Phi(\hat{q}_s^n),\Phi(q_s^\infty)) \\
\end{aligned}
$$

Suppose $\mathcal{W}_1(\hat{q}_s^n,q_s^\infty) \rightarrow 0$ as $n\rightarrow \infty$, indicating that $\hat{q}_s^n$ weakly converges to $q_s^\infty$. 
Then for any fixed $v\in \X$, $h_s(v) \rightarrow 0$ as $n \rightarrow \infty$. 
% Since $\X$ is compact
By the Arzel\`a-Ascoli Theorem, 
the function family $\{ h_s \}_{n=1}^\infty$ with the same Lipschitz constant $2 \L$ is uniformly bounded.
Therefore, it's obtained that $\E_{v\sim q_s^\infty}|h(v)| \rightarrow 0$ as $n \rightarrow \infty$. Finally, we can conclude that
$$
\lim\limits_{n\rightarrow \infty} \mathcal{W}_1(\hat{q}_s^n,q_s^\infty) = 0 
\Rightarrow 
\lim\limits_{n\rightarrow \infty} \mathcal{W}_1(\Phi(\hat{q}_s^n),\Phi(q_s^\infty)) = 0
$$

Now that we have $\lim_{n\to \infty} \mathcal{W}_1(\hat{q}_0^n,\hat{q}_0^\infty) =  0$, 
with mathematical induction, it can be concluded that for any finite iteration $s$,
$\lim_{n\to \infty} \mathcal{W}_1(\hat{q}_s^n,q_s^\infty) = 0.$
\end{proof}

\section{Proof of Proposition \ref{thm:convergence}}
\begin{proof}
We denote the update of our algorithm by $T_{q,p}(x) = x + \epsilon \E_{y \sim q}[\stein_p^y \odot \vv k(x,y)]$ and the transformation of probability distributions by $\Phi : q \mapsto \Phi(q)$ where $\Phi(q)$ is defined to be the distribution of variable $T_{q,p}(x)$ with $x \sim q$.
% For brevity, let $\phi = \phi^*_{q_s^\infty,p}$ and $T := T_{q_s,p}$ where $T_{q_s,p}(x) = x + \epsilon \phi^*_{q_s^\infty,p}(x)$. 

For a properly small $\epsilon$, the update $T_{q,p}$ is invertible for any two distributions $q$ and $p$.
Then we have the following observation on the difference of KL divergence.
$$
\begin{aligned}
& \KL(q_{s+1}^\infty~||~p) - \KL(q_s^\infty~||~p)\\
% =& \KL(\Phi(q_s^\infty)~||~p) - \KL(q_s^\infty~||~p)\\
=& \KL(q_s^\infty ~||~ \Phi^{-1}(p)) - \KL(q_s^\infty ~||~ p)\\
=& -\E_{x\sim q_s^\infty} [ \log p(T_{q_s^\infty, p}(x)) + \\
&~~~~~~~~~~~~\log \det (\nabla T_{q_s^\infty, p}(x)) - \log p(x))]
\end{aligned}
$$

Similarly to the proof of Theorem 4.3 in \citet{2017arXiv170407520L}, 
we can obtain that the difference between KL divergences 
is bounded by the Stein discrepancy in the following way.
Recall that $\phi_i^*(x) = \E_{x \sim q}[ \stein_p^{x_i}  k_i(x,\cdot)]$ is the optimal update of the $i^{th}$ coordinate defined in Theorem \ref{thm:optimal}.
$$
\begin{aligned}
& \KL(q_{s+1}^\infty~||~p) - \KL(q_s^\infty~||~p)\\
\leqslant& -\epsilon \E_{x \sim q_s^\infty}[\nabla_x \log p(x) \phi^*(x)] +
% &\quad\quad 
\frac{\epsilon^2}{2} M_1 \E_{x\sim q_s^\infty}||\phi^*(x)||_2^2 \\
& \quad \quad - \epsilon \E_{x\sim q_s^\infty} [ \nabla \cdot \phi^*(x)]\\
=& -\epsilon \S(q_s^\infty ~||~ p)^2 + \frac{\epsilon^2}{2}M_1 \E_{x\sim q_s^\infty}||\phi^*(x)||_2^2\\
=& -\epsilon \S(q_s^\infty ~||~ p)^2 + \frac{\epsilon^2}{2}M_1 \sum_{i\in n}\E_{x \sim q}[k_i(x,x)]||\phi^*_{i}||_{\H_{i}}^2 \\
\leqslant& -\epsilon \S(q_s^\infty ~||~ p)^2 + \frac{\epsilon^2}{2}M_1 M_2 \sum_{i \in n}||\phi^*_{i}||_{\H_{i}}^2 \\
=& -\epsilon \S(q_s^\infty ~||~ p)^2(1 - \frac{\epsilon}{2}M_1 M_2)\text{ (by Theorem \ref{thm:optimal}. )}\\
\end{aligned}
$$

For $\epsilon \leqslant \frac{1}{M_1 M_2}$, we obtain our main result
$$
\hspace{-40pt}
\KL(q_{s+1}^\infty ~||~ p) - \KL(q_s^\infty ~||~ p) \leqslant - \frac{\epsilon}{2}\S(q_s^\infty ~||~ p)^2.
$$
\end{proof}
